# Supplementary material for: Promptable Closed-loop Traffic Simulation
Source: arXiv:2409.05863 source file (2024-09-09)
Supplement: Supplementary file 1 [file acc_code.tex]

% \begin{minted}[bgcolor=lightgray, linenos, frame=lines, fontsize=\small]{python}
% class Accelerate(V_Action):
%   def __init__(self, agent_token: str):
%     self.agent_token = agent_token

%   @staticmethod
%   def is_applicable(agent_token: str, scenario, ts: int, duration='3s') -> bool:
%     # Check if agent is accelerating

%     # Rule:
%       # Acceleration:
%         # Average acceleration > SPEEDUP_ACCEL[atype] (default: 1.0 m/s^2)
    
%     agent_info = load_agent_info(agent_token, scenario, ts, duration)
%     if agent_info is None:
%       return False

%     traj_speed = agent_info['traj_speed']
%     avg_accel = np.diff(traj_speed).mean() / scenario.ts_dt

%     # print(avg_accel)
%     atype = agent_info['agent_type']
%     if avg_accel > SPEEDUP_ACCEL[atype]:
%       return True

%     return False
% \end{minted}
